# Supplementary material for: How Powerful are Interest Diffusion on Purchasing Prediction: A Case Study of Taocode
Source: arXiv:2112.14446 source file (2021-12-30)
Supplement: Supplementary file 1 [file appendix.tex]

\clearpage
\appendix
\section{Appendix}
\label{sec:appendix}
\subsection{Notations}
Here we summarize the notations used in our proposed model and experiments.

\subsection{diffusion sub-network constructions}
We formulate the process of constructing the diffusion sub-network for a given query.
